# Supplementary material for: Analyzing Twitter Users' Behavior Before and After Contact by the Internet Research Agency
Source: arXiv:2008.01273 source file (2021-02-15)
Supplement: Supplementary file 1 [file appendix.tex]

%!TEX root = main.tex
\newpage

\section{APPENDIX A}

\begin{table}[hbt!]
\caption{P-values returned from significance testing against the random baseline using the timeline data from 2009-2016. User behavior was found to be significantly different from the random baseline set in all cases. }

\begin{tabular}{|c|c|c|}
\hline
\multicolumn{3}{|c|}{\textbf{Low Follower Count Users (2009-2016)}}                                                                                                     \\ \hline
\textbf{Behavior}                     & \textbf{Responsive} & \textbf{Unresponsive}                                 \\ \hline
Tweet Count                           & $7.96 x 10^{-33}$                                       & $4.2 x 10^{-41}$  \\ \hline
Overall Monthly Sentiment            & $3.11 x 10^{-40}$                                             & $9.06 x 10^{-44}$ \\ \hline
@realDonaldTrump Mention Count        & $3.49 x 10^{-12}$                                          & $8.16 x 10^{-11}$ \\ \hline
@realDonaldTrump Sentiment           & $1.59 x 10^{-8}$                                   & 0.001        \\ \hline
@HillaryClinton Mention Count       & $7.31 x 10^{-6}$                                                & $3.05 x 10^{-5}$  \\ \hline
@HillaryClinton Sentiment          & $2.4 x 10^{-10}$                                           & $2.11 x 10^{-10}$ \\ \hline
\multicolumn{1}{l}{}                                 & \multicolumn{1}{l}{}              & \multicolumn{1}{l}{}              & \multicolumn{1}{l}{}                                                                  & \multicolumn{1}{l}{}              \\ \hline
% \multicolumn{1}{l}{}                                 & \multicolumn{1}{l}{}              & \multicolumn{1}{l}{}              & \multicolumn{1}{l}{}                                                                  & \multicolumn{1}{l}{}              \\ \hline
\multicolumn{3}{|c|}{\textbf{High Follower Count Users (2009-2016)}}                                                                                                    \\ \hline
\textbf{Behavior}                    & \textbf{Responsive}} & \textbf{Unresponsive}                                      \\ \hline
Tweet Count                           & $9.06 x 10^{-44}$                                                            & $9.06 x 10^{-44}$ \\ \hline
Overall Monthly Sentiment              & $7.17 x 10^{-43}$                                                            & $9.06 x 10^{-44}$ \\ \hline
@realDonaldTrump Mention Count         & $1.18 x 10^{-14}$                                                         & $3.86 x 10^{-14}$ \\ \hline
@realDonaldTrump Sentiment             & $3.85 x 10^{-7}$         & 0.019        \\ \hline
@HillaryClinton Mention Count         & $4.02 x 10^{-9}$                                                             & $3.23 x 10^{-7}$  \\ \hline
@HillaryClinton Sentiment             & $2.4 x 10^{-10}$                                                           & $2.11 x 10^{-10}$ \\ \hline
\end{tabular}
\label{table3}
\end{table}
